# Supplementary material for: Abolitionist Networks: Modeling Language Change in Nineteenth-Century Activist Newspapers
Source: arXiv:2103.07538 source file (2021-03-12)
Supplement: Supplementary file 1 [file 090appendix.tex]

%%TC:ignore

\begin{appendices}

\section{Newspapers}
To provide some additional context for every newspaper that we considered, we provide some additional description in \autoref{tab:newspapers-description}.
\input{tab-newspaper-descriptions}

\section{Examples of Semantic Changes}
A few examples of words that shift in meaning, with the context in which these words are used are shown in \autoref{tab:semantic-changes-examples}.

\input{tab-semantic-changes}

\begin{comment}

\section{Filtering words}
Our measure of semantic change assigns a score for every word in $\Vcal$. Many words appear as semantic changes but are not genuine changes: function words (e.g. \example{the}, \example{for}), named entities (e.g. \example{toronto}, \example{blakley}), infrequent words (e.g. \example{stuccoed}, \example{barrows}), \etc{} undergo changes in the embedding space but are unlikely to have changed in meaning. We use several heuristics to remove such words from the set of genuine semantic changes.

\begin{table}[H]
    \centering
    \begin{tabular}{l|p{6cm}|l}
       \toprule
        Filter type & Description & Examples \\
        \midrule
        \multirow{2}{*}{Typos or initials} & Words that end in ``-'' & \\
        & Words with length $\leq 2$ & \\
        \multirow{4}{*}{Infrequent words} & Words that have zero count for $5$ or more epochs & Y\\
        & Words that appear in fewer than $4$ sources & Y\\
        & Words that appear fewer than $3$ times in any epoch in which the word changed & Y\\
        \bottomrule
    \end{tabular}

        %Words that appear fewer than 3 times in any epoch in which the word changed & \\
        %Words whose 7 or more neighbors appear fewer than 3 times in any epoch in which the word changed & \\
        %\bottomrule
    %\end{tabular}
    \caption{Heuristic rules for filtering out words }
    \label{tab:filtering-rules}
\end{table}
\end{comment}
%\section{Some More Notation}
\end{appendices}

%%TC:endignore
